# Supplementary material for: Mediated interactions and photon bound states in an exciton-polariton mixture
Source: arXiv:2003.04659 source file (2020-05-13)
Supplement: Supplementary file 1 [file Supplemental_LQ17125.pdf]

# Supplemental Material: Strong mediated polariton interactions and photon dimers

A. Camacho-Guardian[1], M. Bastarrachea-Magnani[1] and G. M. Bruun[1,2]
[1]Department of Physics and Astronomy, Aarhus University, Ny Munkegade, 8000 Aarhus C, Denmark and
[2]Shenzhen Institute for Quantum Science and Engineering and Department of Physics,
Southern University of Science and Technology, Shenzhen 518055, China
(Dated: May 6, 2020)

## I. BOGOLIUBOV THEORY AND SINGLE QUASIPARTICLE PROPERTIES

### A. Bogoliubov approach

We briefly describe the Bogoliubov theory for the exciton-polaritons forming the background. For simplicity we omit the polarisation index $\sigma$. The Hamiltonian of the single specie (majority) is given by

$$\hat{H} = \hat{H}_{xc} + \hat{H}_{xx} + \hat{H}_f, \tag{S1}$$

where the first term comprises the light-matter interaction

$$\hat{H}_{xc} = \sum_i \sum_{\mathbf{k}} \hat{a}^\dagger_{i,\mathbf{k}} \mathbf{h}^0_{ij} \hat{a}_{j,\mathbf{k}}, \tag{S2}$$

$\hat{a}_{i,\mathbf{k}}$ ($\hat{a}^\dagger_{i,\mathbf{k}}$) are the annihilation (creation) operators of the excitons ($i = x$) and photons ($i = c$), respectively, in the $\mathbf{k}$ momentum state, and

$$\mathbf{h}^0 = \begin{pmatrix} \varepsilon^x_{\mathbf{k}} & \Omega/2 \\ \Omega/2 & \varepsilon^c_{\mathbf{k}} \end{pmatrix}. \tag{S3}$$

The non-linear part of the Hamiltonian contains the interactions between co-circular excitons that come from a contact repulsive potential. It reads,

$$\hat{H}_{xx} = \frac{1}{2} \sum_{\mathbf{q},\mathbf{k},\mathbf{k}'} g_{\uparrow\uparrow} \left( \hat{a}^\dagger_{x,\mathbf{k}+\mathbf{q}} \hat{a}^\dagger_{x,\mathbf{k}'-\mathbf{q}} \hat{a}_{x,\mathbf{k}'} \hat{a}_{x,\mathbf{k}} \right) \tag{S4}$$

where $g_{\uparrow\uparrow}$ is the interaction between the co-circular excitons.

Additionally, we consider a driving term to the $\uparrow$ excitons by taking the quasi-mode coupling approximation valid for high-quality mirrors.

$$\hat{H}_f = \sum_{\mathbf{k}} \Omega_f \left( \hat{a}^\dagger_{x,\mathbf{k}} F + F^* \hat{a}_{x,\mathbf{k}} \right). \tag{S5}$$

Here, $\Omega_f$ is the quasi-mode coupling, and

$$F(\mathbf{x}, t) = |F_{\rm pu}| \exp\left[ i \left( \mathbf{k}_{\rm pu} \cdot \mathbf{x} - \omega_{\rm pu} t/\hbar \right) \right], \tag{S6}$$

is the external electric field driving the microcavity, being $\mathbf{k}_{pu}$, $\omega_{pu}$ and $|F_{pu}|$ the momentum, frequency and amplitude of the driving field, respectively. Because we are working in the momentum representation, we take the Fourier transform of the driving

$$F = \int d\mathbf{x}\, F(\mathbf{x}, t) e^{-i\mathbf{k}\cdot\mathbf{x}} = |F_{\rm pu}| e^{-i\omega_{\rm pu} t/\hbar} \delta_{\mathbf{k},\mathbf{k}_{\rm pu}}, \tag{S7}$$

We consider that $\mathbf{k}_{\rm pu} = 0$. The overall effect of this term is to adjust the chemical potential of the $\uparrow$ excitons in the BEC by $\omega_{\rm pu}$, which is set to be $\omega_{\rm pu} = \varepsilon^0_{\rm LP}(\mathbf{0})$. In the absence of exciton-exciton interactions the light-matter Hamiltonian $H_{xc}$ can be diagonalized leading to the polariton quasiparticles

$$\begin{pmatrix} \hat{a}_{x,\mathbf{k}} \\ \hat{a}_{c,\mathbf{k}} \end{pmatrix} = \begin{pmatrix} \mathcal{C}_{\mathbf{k}} & -\mathcal{S}_{\mathbf{k}} \\ \mathcal{S}_{\mathbf{k}} & \mathcal{C}_{\mathbf{k}} \end{pmatrix} \begin{pmatrix} \hat{L}_{\mathbf{k}} \\ \hat{U}_{\mathbf{k}} \end{pmatrix} \tag{S8}$$

where $\hat{L}_{\mathbf{k}}$ ($\hat{U}_{\mathbf{k}}$) are the new bosonic lower-polariton (upper) annihilation operator, and the so-called Hopfield coefficients are $\mathcal{C}^2_{\mathbf{k}}$ and $\mathcal{S}^2_{\mathbf{k}} = 1 - \mathcal{C}^2_{\mathbf{k}}$ given in the main text. After applying the Hopfield transformation and dropping the upper-polariton terms we obtain

$$\hat{H} = \sum_{\mathbf{k}} \left[\varepsilon^0_{\mathrm{LP}}(\mathbf{k})\hat{L}^\dagger_{\mathbf{k}}\hat{L}_{\mathbf{k}} + \Omega_f \mathcal{S}_{\mathbf{k}}\left(\hat{L}^\dagger_{\mathbf{k}}F + F^*\hat{L}_{\mathbf{k}}\right)\right] + \frac{g_{\uparrow\uparrow}}{2}\sum_{\mathbf{q},\mathbf{k},\mathbf{k}'} \mathcal{C}_{\mathbf{k}+\mathbf{q}}\mathcal{C}_{\mathbf{k}'-\mathbf{q}}\mathcal{C}_{\mathbf{k}'}\mathcal{C}_{\mathbf{k}}\hat{L}^\dagger_{\mathbf{k}+\mathbf{q}}\hat{L}^\dagger_{\mathbf{k}'-\mathbf{q}}\hat{L}_{\mathbf{k}'}\hat{L}_{\mathbf{k}}. \tag{S9}$$

Now, we introduce new annihilation (and creation) operators in the rotating frame $\hat{l}_{\mathbf{k}} = \hat{L}_{\mathbf{k}} \exp\left(-i\omega_{\mathrm{pu}}t/\hbar\right)$. In this rotating frame we employ the canonical Bogoliubov approximation and write the Hamiltonian as

$$\hat{H} = E_0 + \sum_{\mathbf{q}\neq\mathbf{k}_{pu}} E^{\mathrm{BEC}}_{\mathbf{q}}\hat{\beta}^\dagger_{\mathbf{q}}\hat{\beta}_{\mathbf{q}}, \tag{S10}$$

here $\hat{\beta}$ denote the Bogoliubov operators, and the coherence factors of the canonical transformation are given by

$$u_{\mathbf{q}}, v_{\mathbf{q}} = \sqrt{\frac{1}{2}\left(\frac{\varepsilon^0_{\mathrm{LP}}(\mathbf{q}) - \omega_{\mathrm{pu}} + 2g_{\uparrow\uparrow}n_b\mathcal{C}^2_0\mathcal{C}^2_{\mathbf{q}}}{E^{\mathrm{BEC}}_{\mathbf{q}}} \pm 1\right)}, \tag{S11}$$

with a dispersion

$$E^{BEC}_{\mathbf{q}} = \sqrt{\left(\varepsilon^0_{\mathrm{LP}}(\mathbf{q}) - \omega_{\mathrm{pu}} + 2g_{\uparrow\uparrow}n_b\mathcal{C}^2_0\mathcal{C}^2_{\mathbf{q}}\right)^2 - g^2_{\uparrow\uparrow}n^2_b\mathcal{C}^4_0\mathcal{C}^4_{\mathbf{q}}}, \tag{S12}$$

being $n_b$ the density of lower-polaritons. We note that the nonequilibrium Bogoliubov mode becomes gapped [S1]. The Green's function describing the BEC are given by

$$G^{(\mathrm{LP})}_{11}(\mathbf{q},z) = G^{(\mathrm{LP})}_{22}(\mathbf{q},-z) = \left(\frac{u^2_{\mathbf{q}}}{z - E^{BEC}_{\mathbf{q}}} - \frac{v^2_{\mathbf{q}}}{z + E^{BEC}_{\mathbf{q}}}\right),\; G^{(\mathrm{LP})}_{12}(\mathbf{q},-z) = G^{(\mathrm{LP})}_{21}(\mathbf{q},-z) = \left(\frac{u_{\mathbf{q}}v_{\mathbf{q}}}{z + E^{BEC}_{\mathbf{q}}} - \frac{v_{\mathbf{q}}u_{\mathbf{q}}}{z - E^{BEC}_{\mathbf{q}}}\right). \tag{S13}$$

### B. Quasiparticle properties

For a single impurity, the quasiparticle properties can be determined following the approach in [S2]

$$\mathcal{G}^{\downarrow}(\mathbf{k},\omega) = \left[(\mathcal{G}^{\downarrow}_0(\mathbf{k},\omega))^{-1} - \Sigma^{\downarrow}(\mathbf{k},\omega)\right]^{-1}. \tag{S14}$$

The impurity propagator is the 2x2 matrix given by

$$\mathcal{G}^{\downarrow}(\mathbf{k},\omega) = \begin{pmatrix} \mathcal{G}_{xx} & \mathcal{G}_{xc} \\ \mathcal{G}_{cx} & \mathcal{G}_{cc} \end{pmatrix}, \tag{S15}$$

where the diagonal terms $\mathcal{G}_{xx}(\mathbf{k},\omega)$ and $\mathcal{G}_{cc}(\mathbf{k},\omega)$, account for the excitonic and photonic parts of the impurity. The ideal propagator of the impurity is a diagonal matrix such that $\mathrm{diag}((\mathcal{G}^{\downarrow}_0(\mathbf{k},\omega))^{-1}) = (\omega - \varepsilon^x_{\mathbf{k}}, \omega - \varepsilon^c_{\mathbf{k}})$. We employ the scattering matrix for counter-polarised excitons, which can be written as $\mathcal{T}^{-1}(\mathbf{p},z) = \Pi(\mathbf{0},\varepsilon_{\uparrow\downarrow}) - \Pi(\mathbf{p},z)$, and includes the bi-exciton energy. We calculate the self-energy as

$$\Sigma^{\downarrow}(\mathbf{k},\omega) = \begin{pmatrix} \Sigma_{xx}(\mathbf{k},\omega) & \Omega/2 \\ \Omega/2 & 0 \end{pmatrix}, \tag{S16}$$

where the exciton-exciton self-energy is given explicitly by

$$\Sigma_{xx}(\mathbf{k},\omega) = n_{\mathrm{LP}}\mathcal{C}^2_0\mathcal{T}(\mathbf{k},\omega) + \frac{1}{V}\sum_{\mathbf{q}} v^2_{\mathbf{q}}\mathcal{C}_{\mathbf{q}}\mathcal{C}_{-\mathbf{q}}\mathcal{T}(\mathbf{k}+\mathbf{q},\omega - E_{\mathbf{q}}), \tag{S17}$$

for the Dyson equation we identify the quasiparticle properties, that is

$$\mathrm{Re}G^{\downarrow}(\mathbf{p},\varepsilon_{\mathbf{k}})^{-1} = 0 \tag{S18}$$

$$Z_{\mathbf{k}} = \left.\frac{1}{\partial_\omega G^{\downarrow}(\mathbf{p},\omega)}\right|_{\omega=\varepsilon_{\mathbf{k}}}.$$

While the former determines the quasiparticle branches $\varepsilon_{\mathbf{k}}$ in Fig. 2 (main text) the latter defines the quasiparticle residue. As shown in [S2] the strong light-matter coupling and the Feshbach physics yield a rich landscape of quasiparticle features. In Fig. S1 (a) we compare the light transmission for a single impurity [S2] and compare with the results of the main text for $n = 0.15 n_B$ Fig. S1(b). For comparison purposes we employ the same vertical axis as in Ref. [S2]

In Fig. S1 we show the light transmission in the limit of a single impurity. For comparison purposes between the single impurity discussed in Ref. [S2] (left) and the main text we show the light transmission for $n = 0.15 n_B$(right) for a fixed polaritonic density $n_B$.

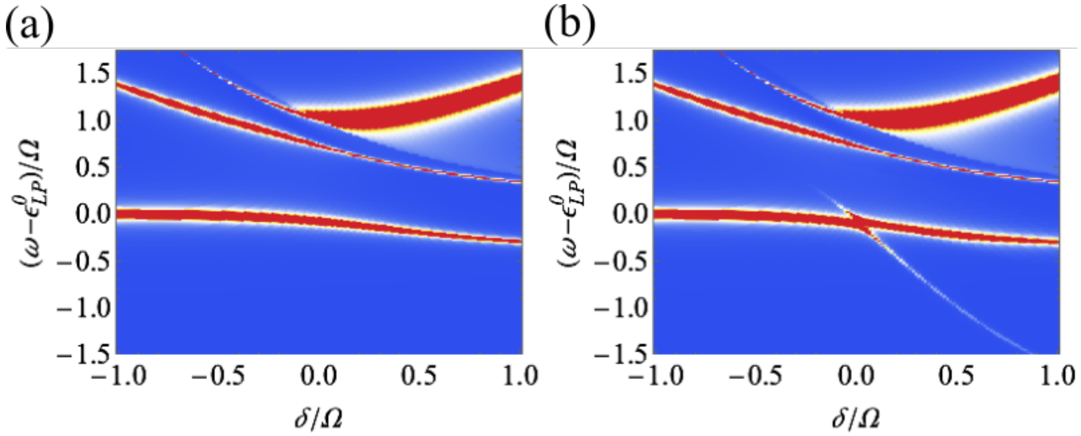


FIG. S1: Light transmission for a single impurity (a) and for a finite density of impurities including the mediated interaction between the polaritons (b).

## II. MEDIATED INTERACTION

The mediated interaction between excitons describing the exchange of sound-modes between the ↓ exciton-polaritons is given by

$$V(p,p';q) = n_B \mathcal{C}_0^2 \mathcal{C}_{\mathbf{q}}^2 \Big[\mathcal{T}(p+q/2) G_{11}^{(\mathrm{LP})}(q) \mathcal{T}(p+q/2) + \mathcal{T}(p-q/2) G_{22}^{(\mathrm{LP})}(q) \mathcal{T}(p-q/2) + \mathcal{T}(p+q/2) G_{12}^{(\mathrm{LP})}(q) \mathcal{T}(p-q/2) + \mathcal{T}(p-q/2) G_{21}^{(\mathrm{LP})}(q) \mathcal{T}(p+q/2)\Big], \tag{S19}$$

which can be written in a compact matrix form as shown in Eq. 2 (main text). In the case where the interaction between anti-parallel polarised exciton is energy independent $\mathcal{T}(p) \approx g_{\uparrow\downarrow}$ the induced interaction depends only on the transferred energy-momentum $V(p,p';q) = V(q)$. Furthermore, for a purely atomic BEC and within the static limit the induced interaction takes the form of

$$V(\mathbf{q}) = n_B \frac{2}{\frac{q^2}{2m} + 2 g_{\uparrow\downarrow} n_B}, \tag{S20}$$

the range of the potential is therefore characterised by $\xi \propto 1/\sqrt{2 m g_{\uparrow\downarrow} n_B}$in agreement with [S3]. As explained above, the coupling to light modifies the Bogoliubov spectrum, in addition, the interaction in Eq. S19 accounts for the modified Hopfield coefficients as well as the normalisation factors due to the quasiparticle residues. Note that the photonic nature of the direct and mediated scattering is encoded then in the BEC Green's function, scattering matrix $\mathcal{T}$, and the exciton component of the polaron-polaritons and, as shown in Eq. (3) of the main text, the light-matter coupling leads to different results when compared to pure matter-quasiparticle scattering.

The Bethe-Salpeter equation in Eq. (4) (main text) is evaluated after a pole expansion for the $G(\mathbf{p}, z)$ propagator and by neglecting retardation effects in Eq. S19. The pole expansion takes into account the reduction of the quasiparticle pole which is relevant for the attractive polaron that cedes spectral weight to the repulsive branch as the momentum $\mathbf{k}$ increases in magnitude. On the other hand, due to the small mass of polaritons, the speed of sound of the BEC is of the order of $c_s = \sqrt{n_b g_{\uparrow\downarrow}/m_{\mathrm{LP}}} \approx 10^6$m/s, therefore, the density oscillations within the medium propagates much faster

than in an atomic gas [S4]. We expect an efficient exchange of Bogoliubov modes within the BEC, and our theory to be accurate when $\delta v/c_s < 1$, where $\delta v = \sqrt{(E - 2\varepsilon_{\mathrm{LP}}(\mathbf{0}))/m_{\mathrm{LP}}}$, which turns to be indeed the case for the onset of the two-body body bound states. Finally, details on the Bethe-Salpeter equation can be found in [S5], which has been extended to include the polaritonic features due to the strong light-matter coupling.

[S1] I. Carusotto and C. Ciuti, Rev. Mod. Phys. **85**, 299 (2013), URL https://link.aps.org/doi/10.1103/RevModPhys.85.299.

[S2] M. A. Bastarrachea-Magnani, A. Camacho-Guardian, M. Wouters, and G. M. Bruun, Phys. Rev. B **100**, 195301 (2019), URL https://link.aps.org/doi/10.1103/PhysRevB.100.195301.

[S3] L. Viverit, C. J. Pethick, and H. Smith, Phys. Rev. A **61**, 053605 (2000), URL https://link.aps.org/doi/10.1103/PhysRevA.61.053605.

[S4] A. Amo, J. Lefrère, S. Pigeon, C. Adrados, C. Ciuti, I. Carusotto, R. Houdré, E. Giacobino, and A. Bramati, Nature Physics **5**, 805 EP (2009), URL https://doi.org/10.1038/nphys1364.

[S5] A. Camacho-Guardian, L. A. Peña Ardila, T. Pohl, and G. M. Bruun, Phys. Rev. Lett. **121**, 013401 (2018), URL https://link.aps.org/doi/10.1103/PhysRevLett.121.013401.
